# Supplementary material for: Driven anisotropic diffusion at boundaries: noise rectification and particle sorting
Source: arXiv:1706.01660 ancillary file (2017-07-12)
Supplement: Supplementary file 1 [file supplementary.pdf]

# Supplementary Material
# Driven anisotropic diffusion at boundaries: noise rectification and particle sorting

Stefano Bo[1] and Ralf Eichhorn[1]
[1]*Nordita, Royal Institute of Technology and Stockholm University, Roslagstullsbacken 23, SE-106 91 Stockholm, Sweden*
(Dated: July 4, 2017)

## I. SOLUTION

### A. Model

The problem we are interested in is described by a Fokker Planck equation with constant symmetric diffusion tensor and constant drift as in eq. (1) in the main text,

$$\frac{\partial p}{\partial t} = -\frac{\partial}{\partial x_i}\left(v_i - \frac{\partial}{\partial x_j} D_{ij}\right) p \equiv \mathcal{L}^\dagger p \equiv -\frac{\partial}{\partial x_i} J_i \,, \tag{S1}$$

where we have introduced the forward operator

$$\mathcal{L}^\dagger = -\frac{\partial}{\partial x_i}\left(v_i - \frac{\partial}{\partial x_j} D_{ij}\right) , \tag{S2}$$

and the probability flux

$$J_i = v_i p - \frac{\partial}{\partial x_j} D_{ij} p \,, \tag{S3}$$

and summation over repeated indices is understood. We consider the 3D case with a plain surface (reflecting boundary) set at $x_3 = 0$. The presence of the boundary implies the condition

$$\Big[J_3\Big]_{x_3=0} = \left[v_3 p - \frac{\partial}{\partial x_j} D_{3j} p\right]_{x_3=0} = 0 \,, \tag{S4}$$

as in eq. (2) in the main text.

### B. Free diffusion

Without the no-flux boundary condition (S4), free diffusion in 3D has a trivariate Gaussian propagator,

$$p_{\text{free}}(x_1, x_2, x_3) = \frac{1}{\sqrt{|\mathsf{D}|(4\pi t)^3}}\, e^{-\frac{1}{4t}\left(x_i - x_i^{(0)} - v_i t\right)\bar{D}_{ij}\left(x_j - x_j^{(0)} - v_j t\right)} \equiv \frac{1}{\sqrt{|\mathsf{D}|(4\pi t)^3}}\, e^{-\frac{1}{4t}(x_i-\mu_i)\bar{D}_{ij}(x_j-\mu_j)} \,, \tag{S5}$$

where $\bar{D}_{ij} \equiv \left(\mathsf{D}^{-1}\right)_{ij}$ denotes the entries of the inverse diffusion tensor and $\mu_i \equiv x_i^{(0)} + v_i t$. The conditional density

$$p_{\text{free}}(x_1, x_2 | x_3) = \frac{p_{\text{free}}(x_1, x_2, x_3)}{p_{\text{free}}(x_3)} = \frac{1}{\sqrt{|\tilde{\mathsf{D}}|(4\pi t)^2}}\, e^{-\frac{1}{4t}(x_j-\tilde{\mu}_j)\left(\tilde{\mathsf{D}}^{-1}\right)_{jk}(x_k-\tilde{\mu}_k)} \tag{S6}$$

(with $j, k$ running from 1 to 2) is a two-dimensional Gaussian with mean

$$\tilde{\mu}_j = \mu_j + \frac{D_{3j}}{D_{33}}(x_3 - \mu_3) \tag{S7}$$

and covariance matrix proportional to the Schur complement of $D_{33}$ in $\mathsf{D}$,

$$2\tilde{\mathsf{D}}t = \frac{2t}{D_{33}}\begin{pmatrix} D_{11}D_{33} - D_{13}^2 & D_{12}D_{33} - D_{23}D_{13} \\ D_{12}D_{33} - D_{23}D_{13} & D_{22}D_{33} - D_{23}^2 \end{pmatrix} . \tag{S8}$$

The part

$$p_{\rm free}(x_3) = \frac{1}{\sqrt{4\pi D_{33}t}}\, e^{-\frac{\left(x_3 - x_3^{(0)} - v_3 t\right)^2}{4D_{33}t}} \tag{S9}$$

represents free diffusion (no boundaries) in one dimension with drift $v_3$ and diffusion coefficient $D_{33}$. It obeys the one-dimensional Fokker Planck equation (in $x_3$) and consequently the full one

$$\frac{\partial p_{\rm free}(x_3)}{\partial t} = \mathcal{L}^\dagger p_{\rm free}(x_3)\,. \tag{S10}$$

### C. Diffusion with reflecting boundary

The 3-dimensional solution of eq. (S1) (for a delta-distributed initial density $p(\boldsymbol{x}, 0) = \delta(\boldsymbol{x} - \boldsymbol{x}^{(0)})$, assuming $x_3^{(0)} > 0$) with boundary condition (S4), can be built from the one-dimensional solution of diffusion in front of a reflecting boundary derived by Smoluchowski [6, 7]. As we shall verify below, the solution $p(x_1, x_2, x_3)$ of (S1) on the half-space $x_3 \geq 0$ with the reflecting boundary condition (S4) retains the (conditional) free diffusion in the $x_1$ and $x_2$ components $p_{\rm free}(x_1, x_2|x_3)$, while the unconstrained $x_3$ component is replaced by the solution $p(x_3)$ for one-dimensional diffusion on the half-line $x_3 > 0$ with a reflecting boundary at $x_3 = 0$ [6, 7],

$$\boxed{p(x_1, x_2, x_3) = p_{\rm free}(x_1, x_2|x_3)p(x_3)}\,. \tag{S11}$$

The explicit form of $p(x_3)$ for one-dimensional diffusion on the half-line, as derived by Smoluchowski [6], reads

$$p(x_3) = p_{\rm free}(x_3) + \frac{1}{\sqrt{4\pi D_{33}t}}\, e^{-\frac{v_3}{D_{33}}x_3^{(0)}}\, e^{-\frac{\left(x_3 + x_3^{(0)} - v_3 t\right)^2}{4D_{33}t}} - \frac{v_3}{2D_{33}} e^{\frac{v_3}{D_{33}}x_3}\, \mathrm{erfc}\left[\frac{x_3 + x_3^{(0)} + v_3 t}{\sqrt{4D_{33}t}}\right]\,, \tag{S12}$$

where $p_{\rm free}(x_3)$ is the same expression for free diffusion as in eq. (S9), but now applied only to the half-line $x_3 \in [0, +\infty)$, and where $\mathrm{erfc}(x)$ denotes the complementary error function. With (S6), the full time-dependent solution of our problem (S1), (S4) therefore reads (for sake of clarity we here spell out the sum in the exponent explicitly)

$$\begin{aligned}
p(x_1, x_2, x_3) = {} & \frac{1}{\sqrt{|\mathsf{D}|(4\pi t)^3}}\, e^{-\frac{1}{4t}\sum_{j,k=1}^{2}\left(x_j - x_j^{(0)} - v_j t - \frac{D_{3j}}{D_{33}}\left(x_3 - x_3^{(0)} - v_3 t\right)\right)\left(\tilde{\mathsf{D}}^{-1}\right)_{jk}\left(x_k - x_k^{(0)} - v_k t - \frac{D_{3k}}{D_{33}}\left(x_3 - x_3^{(0)} - v_3 t\right)\right)} \\
& \times \left( e^{-\frac{\left(x_3 - x_3^{(0)} - v_3 t\right)^2}{4D_{33}t}} + e^{-\frac{v_3}{D_{33}}x_3^{(0)}}\, e^{-\frac{\left(x_3 + x_3^{(0)} - v_3 t\right)^2}{4D_{33}t}} - \sqrt{\frac{\pi t}{D_{33}}} v_3\, e^{\frac{v_3}{D_{33}}x_3}\, \mathrm{erfc}\left[\frac{x_3 + x_3^{(0)} + v_3 t}{\sqrt{4D_{33}t}}\right]\right) \\
= {} & \frac{1}{\sqrt{|\mathsf{D}|(4\pi t)^3}}\, e^{-\frac{1}{4t}\sum_{i,j=1}^{3}\left(x_i - x_i^{(0)} - v_i t\right)\bar{D}_{ij}\left(x_j - x_j^{(0)} - v_j t\right)} \\
& + \frac{1}{\sqrt{|\mathsf{D}|(4\pi t)^3}}\, e^{-\frac{1}{4t}\sum_{j,k=1}^{2}\left(x_j - x_j^{(0)} - v_j t - \frac{D_{3j}}{D_{33}}\left(x_3 - x_3^{(0)} - v_3 t\right)\right)\left(\tilde{\mathsf{D}}^{-1}\right)_{jk}\left(x_k - x_k^{(0)} - v_k t - \frac{D_{3k}}{D_{33}}\left(x_3 - x_3^{(0)} - v_3 t\right)\right)} \\
& \times \left( e^{-\frac{v_3}{D_{33}}x_3^{(0)}}\, e^{-\frac{\left(x_3 + x_3^{(0)} - v_3 t\right)^2}{4D_{33}t}} - \sqrt{\frac{\pi t}{D_{33}}} v_3\, e^{\frac{v_3}{D_{33}}x_3}\, \mathrm{erfc}\left[\frac{x_3 + x_3^{(0)} + v_3 t}{\sqrt{4D_{33}t}}\right]\right)\,.
\end{aligned} \tag{S13}$$

### D. Properties of the Smoluchowski solution $p(x_3)$ in 1 dimension

The Smoluchowski solution $p(x_3)$ satisfies the one-dimensional Fokker Planck equation (in $x_3$) and consequently the full one,

$$\frac{\partial p(x_3)}{\partial t} = \mathcal{L}^\dagger p(x_3)\,, \tag{S14}$$

and the no boundary flux condition in one dimension,

$$\left[v_3 p(x_3) - \frac{\partial}{\partial x_3} D_{33} p(x_3)\right]_{x_3=0} = 0\,. \tag{S15}$$

It is normalized over $x_3 \in [0, +\infty)$. We can easily check the normalization by direct integration. For the first two terms we have

$$\int_0^\infty \mathrm{d}x_3\, p_{\mathrm{free}}(x_3) = \frac{1}{\sqrt{4\pi D_{33} t}} \int_0^\infty \mathrm{d}x_3\, e^{-\frac{\left(x_3 - x_3^{(0)} - v_3 t\right)^2}{4D_{33}t}} = 1 - \frac{1}{2}\,\mathrm{erfc}\left[\frac{x_3^{(0)} + v_3 t}{\sqrt{4D_{33}t}}\right] \tag{S16}$$

$$\frac{1}{\sqrt{4\pi D_{33} t}}\, e^{-\frac{v_3}{D_{33}} x_3^{(0)}} \int_0^\infty \mathrm{d}x_3\, e^{-\frac{\left(x_3 + x_3^{(0)} - v_3 t\right)^2}{4D_{33}t}} = \frac{1}{2} e^{-\frac{v_3}{D_{33}} x_3^{(0)}}\,\mathrm{erfc}\left[\frac{x_3^{(0)} - v_3 t}{\sqrt{4D_{33}t}}\right] . \tag{S17}$$

For the third term, we can make use of the relation

$$\int \mathrm{d}x\, e^{bx}\,\mathrm{erfc}[ax] = \frac{1}{b} e^{bx}\,\mathrm{erfc}\,[ax] - \frac{1}{b} e^{\frac{b^2}{4a^2}}\,\mathrm{erfc}\left[ax - \frac{b}{2a}\right] , \tag{S18}$$

which follows from integration by parts [9]. We then get

$$-\frac{v_3}{2D_{33}} \int_0^\infty \mathrm{d}x_3\, e^{\frac{v_3}{D_{33}} x_3}\,\mathrm{erfc}\left[\frac{x_3 + x_3^{(0)} + v_3 t}{\sqrt{4D_{33}t}}\right] = \frac{1}{2}\left\{\mathrm{erfc}\left[\frac{x_3^{(0)} + v_3 t}{\sqrt{4D_{33}t}}\right] - e^{\frac{v_3}{D_{33}} x_3^{(0)}}\,\mathrm{erfc}\left[\frac{x_3^{(0)} - v_3 t}{\sqrt{4D_{33}t}}\right]\right\} . \tag{S19}$$

Summing up these three contributions we find normalization 1.

## E. Normalization of (S11)

The normalization of the solution (S11) is ensured by the fact that the conditional probability is normalized over the plane $x_1 \in (-\infty, +\infty)$, $x_2 \in (-\infty, +\infty)$ and that $p(x_3)$ is normalized over $x_3 \in [0, +\infty)$

$$\int_{-\infty}^\infty \mathrm{d}x_1 \int_{-\infty}^\infty \mathrm{d}x_2 \int_0^\infty \mathrm{d}x_3\, p_{\mathrm{free}}(x_1, x_2|x_3) p(x_3) = \int_0^\infty \mathrm{d}x_3\, p(x_3) = 1 . \tag{S20}$$

## F. Proof that (S11) solves the Fokker-Planck equation with no flux boundary condition

We now verify that (S11) is a solution of the Fokker Planck equation with no flux across the surface. Exploiting the symmetry of the diffusion tensor and that $p(x_3)$ does not depend on $x_1$, $x_2$, we can write eq. (S1) as

$$\begin{aligned}
\frac{\partial p_{\mathrm{free}}(x_1, x_2|x_3) p(x_3)}{\partial t} &= \mathcal{L}^\dagger p_{\mathrm{free}}(x_1, x_2|x_3) p(x_3) \\
&= p(x_3)\mathcal{L}^\dagger p_{\mathrm{free}}(x_1, x_2|x_3) + p_{\mathrm{free}}(x_1, x_2|x_3)\mathcal{L}^\dagger p(x_3) \\
&\quad + 2\frac{\partial p(x_3)}{\partial x_3}\left(D_{13}\frac{\partial p_{\mathrm{free}}(x_1, x_2|x_3)}{\partial x_1} + D_{23}\frac{\partial p_{\mathrm{free}}(x_1, x_2|x_3)}{\partial x_2} + D_{33}\frac{\partial p_{\mathrm{free}}(x_1, x_2|x_3)}{\partial x_3}\right) \\
&= p(x_3)\mathcal{L}^\dagger p_{\mathrm{free}}(x_1, x_2|x_3) + p_{\mathrm{free}}(x_1, x_2|x_3)\mathcal{L}^\dagger p(x_3) + 2\frac{\partial p(x_3)}{\partial x_3} D_{i3}\frac{\partial p_{\mathrm{free}}(x_1, x_2|x_3)}{\partial x_i} .
\end{aligned} \tag{S21}$$

Explicitly computing the terms multiplying $\frac{\partial p(x_3)}{\partial x_3}$ shows that they vanish. Indeed, exploiting the symmetry of the diffusion tensor, the definition of the conditional probability (S6), and the explicit expressions of free diffusion (S5) and (S9), we find:

$$\begin{aligned}
\frac{\partial p_{\mathrm{free}}(x_1, x_2|x_3)}{\partial x_i} &= \frac{\partial}{\partial x_i}\left(\frac{p_{\mathrm{free}}(x_1, x_2, x_3)}{p_{\mathrm{free}}(x_3)}\right) \\
&= \frac{1}{p_{\mathrm{free}}(x_3)}\left(\frac{\partial p_{\mathrm{free}}(x_1, x_2, x_3)}{\partial x_i} - p_{\mathrm{free}}(x_1, x_2|x_3)\frac{\partial p_{\mathrm{free}}(x_3)}{\partial x_i}\right) \\
&= -\frac{p_{\mathrm{free}}(x_1, x_2|x_3)}{2t}\left[\bar{D}_{ij}(x_j - x_j^{(0)} - v_j t) - \delta_{i3}\frac{x_3 - x_3^{(0)} - v_3 t}{D_{33}}\right] ,
\end{aligned} \tag{S22}$$

so that

$$D_{3i}\frac{\partial p_{\rm free}(x_1,x_2|x_3)}{\partial x_i} = -\frac{p_{\rm free}(x_1,x_2|x_3)}{2t}\left[\left(\mathsf{D}\mathsf{D}^{-1}\right)_{3j}(x_j - x_j^{(0)} - v_j t) - D_{33}\frac{x_3 - x_3^{(0)} - v_3 t}{D_{33}}\right] = 0\,. \tag{S23}$$

We are then left with

$$\frac{\partial p_{\rm free}(x_1,x_2|x_3)p(x_3)}{\partial t} = p(x_3)\mathcal{L}^\dagger p_{\rm free}(x_1,x_2|x_3) + p_{\rm free}(x_1,x_2|x_3)\mathcal{L}^\dagger p(x_3)\,, \tag{S24}$$

requiring

$$p_{\rm free}(x_1,x_2|x_3)\left(\frac{\partial p(x_3)}{\partial t} - \mathcal{L}^\dagger p(x_3)\right) = -p(x_3)\left(\frac{\partial p_{\rm free}(x_1,x_2|x_3)}{\partial t} - \mathcal{L}^\dagger p_{\rm free}(x_1,x_2|x_3)\right)\,. \tag{S25}$$

We know that the one dimensional solution $p(x_3)$ satisfies the Fokker-Planck equation (S14) so that the LHS vanishes. Concerning the RHS, we have to recall that free diffusion is solved by $p_{\rm free}(x_1,x_2,x_3) = p_{\rm free}(x_1,x_2|x_3)p_{\rm free}(x_3)$, i.e.

$$\begin{aligned}\frac{\partial p_{\rm free}(x_1,x_2,x_3)}{\partial t} &= p_{\rm free}(x_3)\mathcal{L}^\dagger p_{\rm free}(x_1,x_2|x_3) + p_{\rm free}(x_1,x_2|x_3)\mathcal{L}^\dagger p_{\rm free}(x_3) + 2\frac{\partial p_{\rm free}(x_3)}{\partial x_3}D_{i3}\frac{\partial p_{\rm free}(x_1,x_2|x_3)}{\partial x_i}\\ &= p_{\rm free}(x_3)\mathcal{L}^\dagger p_{\rm free}(x_1,x_2|x_3) + p_{\rm free}(x_1,x_2|x_3)\mathcal{L}^\dagger p_{\rm free}(x_3)\,,\end{aligned} \tag{S26}$$

which, since $\frac{\partial p_{\rm free}(x_3)}{\partial t} - \mathcal{L}^\dagger p_{\rm free}(x_3) = 0$, implies

$$\frac{\partial p_{\rm free}(x_1,x_2|x_3)}{\partial t} - \mathcal{L}^\dagger p_{\rm free}(x_1,x_2|x_3) = 0\,. \tag{S27}$$

It follows that the RHS of (S25) is indeed zero.

It remains to be checked that the flux in the $x_3$ direction vanishes at the surface $x_3 = 0$:

$$\begin{aligned}J_3 &= v_3 p_{\rm free}(x_1,x_2|x_3)p(x_3) - \frac{\partial}{\partial x_j}D_{3j}p_{\rm free}(x_1,x_2|x_3)p(x_3)\\ &= p_{\rm free}(x_1,x_2|x_3)\underbrace{\left(v_3 p(x_3) - \frac{\partial}{\partial x_3}D_{33}p(x_3)\right)}_{\text{flux of the 1d case}} - p(x_3)\underbrace{\frac{\partial}{\partial x_j}D_{3j}p_{\rm free}(x_1,x_2|x_3)}_{=0}\,.\end{aligned} \tag{S28}$$

For $x_3 = 0$, this is guaranteed by the fact that the Smoluchowski solution (S12) has no flux at the boundary (see (S15)), and by (S23).

## II. AVERAGES AND COVARIANCES

With the full solution given in eq. (S11) it is possible to directly compute the distribution moments. Given the factorized form of the solution, the integrals along direction $x_1$ and $x_2$ are straightforward Gaussian integrals, whereas the ones along $x_3$ involve combinations of error functions, Gaussians and polynomials and require additional care. The idea is to to proceed by computing first the moments of $x_1$ and $x_2$ conditioned on $x_3$, and then average them over the $p(x_3)$ distribution.

For the first moments one has

$$\langle x_i\rangle = \int_0^\infty \mathrm{d}x_3\,\langle x_i|x_3\rangle p(x_3) = \int_0^\infty \mathrm{d}x_3\,\tilde{\mu}_i(x_3)p(x_3) = \mu_i - \frac{D_{3i}}{D_{33}}\mu_3 + \frac{D_{3i}}{D_{33}}\langle x_3\rangle\,, \tag{S29}$$

where (for $i = 1,2$)

$$\langle x_i|x_3\rangle \equiv \int_{-\infty}^\infty \mathrm{d}x_1\int_{-\infty}^\infty \mathrm{d}x_2\,x_i p_{\rm free}(x_1,x_2|x_3)\,. \tag{S30}$$

For the second moments, as we will show below (exploiting the linearity of $\tilde{\mu}_i$ in $x_3$, see (S7)), one has

$$\langle x_i x_j\rangle - \langle x_i\rangle\langle x_j\rangle = 2t\tilde{D}_{ij} + \frac{D_{3i}D_{3j}}{D_{33}^2}\left(\langle x_3^2\rangle - \langle x_3\rangle^2\right)\,, \tag{S31}$$

with $i$, $j$ being 1 or 2. To familiarize with this expression one can check that for the case of free diffusion, where $\langle x_3^2\rangle - \langle x_3\rangle^2 = 2tD_{33}$, one recovers $\langle x_2^2\rangle - \langle x_2\rangle^2 = 2tD_{22}$ by plugging in the explicit expression of $\tilde{D}_{ij}$ from (S8).

Equation (S31) can be derived by splitting the conditional average in a part dependent on $x_3$ and an independent one:

$$\langle x_i|x_3\rangle = \mu_i + \frac{D_{3i}}{D_{33}}(x_3 - \mu_3) = a_i + b_i x_3 \tag{S32}$$

where $a_i = \mu_i - \frac{D_{3i}}{D_{33}}\mu_3$ and $b_i = \frac{D_{3i}}{D_{33}}$. Then

$$\langle x_i\rangle = a_i + b_i\langle x_3\rangle \tag{S33}$$

and

$$\begin{aligned}\langle x_i x_j\rangle - \langle x_i\rangle\langle x_j\rangle &= \int_0^\infty \Big[\langle x_i x_j|x_3\rangle - \langle x_i|x_3\rangle\langle x_j|x_3\rangle + \langle x_i|x_3\rangle\langle x_j|x_3\rangle - \langle x_i\rangle\langle x_j\rangle\Big] p(x_3)\mathrm{d}x_3 \\ &= 2t\tilde{D}_{ij} + \int_0^\infty \langle x_i|x_3\rangle\Big(\langle x_j|x_3\rangle - \langle x_j\rangle\Big)p(x_3)\mathrm{d}x_3 \\ &= 2t\tilde{D}_{ij} + b_i b_j\left(\langle x_3^2\rangle - \langle x_3\rangle^2\right) .\end{aligned} \tag{S34}$$

### A. Time-dependent moments

To explicitly express the moments we need to compute the time-dependent first and second moments of $x_3$, i.e. $\langle x_3\rangle$ and $\langle x_3^2\rangle$. Using (S12) we find

$$\langle x_3\rangle = x_3^{(0)} + v_3 t + \sqrt{\frac{D_{33}t}{\pi}}\, e^{-\frac{\left(x_3^{(0)}+v_3t\right)^2}{4D_{33}t}} + \frac{D_{33}}{2v_3}\, e^{-\frac{v_3}{D_{33}}x_3^{(0)}}\ \mathrm{erfc}\left[\frac{x_3^{(0)} - v_3 t}{\sqrt{4D_{33}t}}\right] - \frac{1}{2}\left(x_3^{(0)} + v_3 t + \frac{D_{33}}{v_3}\right)\mathrm{erfc}\left[\frac{x_3^{(0)} + v_3 t}{\sqrt{4D_{33}t}}\right] . \tag{S35}$$

It follows that

$$\begin{aligned}\langle x_1\rangle = x_1^{(0)} + v_1 t + \frac{D_{31}}{D_{33}}\sqrt{\frac{D_{33}t}{\pi}}\, e^{-\frac{(x_3^{(0)}+v_3t)^2}{4D_{33}t}} + \frac{D_{31}}{2v_3}\, e^{-\frac{v_3}{D_{33}}x_3^{(0)}}\ \mathrm{erfc}\left[\frac{x_3^{(0)} - v_3 t}{\sqrt{4D_{33}t}}\right] \\ - \frac{1}{2}\frac{D_{31}}{D_{33}}\left(x_3^{(0)} + v_3 t + \frac{D_{33}}{v_3}\right)\mathrm{erfc}\left[\frac{x_3^{(0)} + v_3 t}{\sqrt{4D_{33}t}}\right] ,\end{aligned} \tag{S36}$$

$$\begin{aligned}\langle x_2\rangle = x_2^{(0)} + v_2 t + \frac{D_{32}}{D_{33}}\sqrt{\frac{D_{33}t}{\pi}}\, e^{-\frac{(x_3^{(0)}+v_3t)^2}{4D_{33}t}} + \frac{D_{32}}{2v_3}\, e^{-\frac{v_3}{D_{33}}x_3^{(0)}}\ \mathrm{erfc}\left[\frac{x_3^{(0)} - v_3 t}{\sqrt{4D_{33}t}}\right] \\ - \frac{1}{2}\frac{D_{32}}{D_{33}}\left(x_3^{(0)} + v_3 t + \frac{D_{33}}{v_3}\right)\mathrm{erfc}\left[\frac{x_3^{(0)} + v_3 t}{\sqrt{4D_{33}t}}\right] .\end{aligned} \tag{S37}$$

For the time-dependent second moment of $x_3$ we find

$$\begin{aligned}\langle x_3^2\rangle = \left[2D_{33} + v_3\left(x_3^{(0)} + v_3 t\right)\right]\sqrt{\frac{D_{33}t}{\pi v_3^2}}\, e^{-\frac{\left(x_3^{(0)}+v_3t\right)^2}{4D_{33}t}} + \frac{1}{2}\left[2D_{33}t + \left(x_3^{(0)} + v_3 t\right)^2\right]\left(1 + \mathrm{erf}\left[\frac{x_3^{(0)} + v_3 t}{\sqrt{4D_{33}t}}\right]\right) \\ - \left[D_{33} + v_3\left(x_3^{(0)} - v_3 t\right)\right]\frac{D_{33}}{v_3^2}\, e^{-\frac{v_3 x_3^{(0)}}{D_{33}}}\ \mathrm{erfc}\left[\frac{x_3^{(0)} - v_3 t}{\sqrt{4D_{33}t}}\right] + \frac{D_{33}^2}{v_3^2}\,\mathrm{erfc}\left(\frac{x_3^{(0)} + v_3 t}{\sqrt{4D_{33}t}}\right) .\end{aligned} \tag{S38}$$

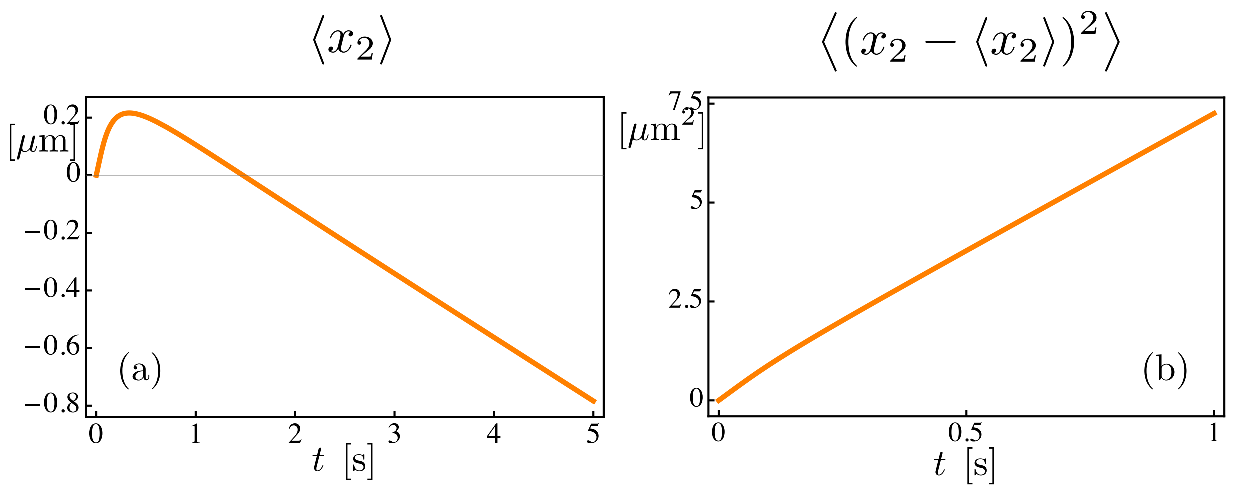


FIG. 1. (a) Average position $\langle x_2 \rangle$ (in $\mu$m following eq. (S37)) for a particle of size $0.25\,\mu$m as a function of time. Note the transient displacement of $\langle x_2 \rangle$ in the direction of the force $f_2$ before the particle comes close enough to the surface for the rectification effect to set in. (b) Variance $\left\langle (x_2 - \langle x_2 \rangle)^2 \right\rangle$ (in $\mu\mathrm{m}^2$ following eq. (S39)) for a particle of size $0.25\,\mu$m as a function of time. In both cases, the parameters are those of figure 1 in the main text: $T = 300\,\mathrm{K}$, $\theta = 0.9\pi$, "synthetic" kinetic temperature $T_{\mathrm{kin}} = T + \sigma^2/(2k_{\mathrm{B}}\gamma_0) = 1000\,\mathrm{K}$ (specified for a reference spherical particle with radius $0.5\,\mu$m), external force $\boldsymbol{f} = (0\,\mathrm{fN}, 7.5\,\mathrm{fN}, -9\,\mathrm{fN})$, and initial position $\boldsymbol{x} = (0, 0, 1\,\mu\mathrm{m})$.

This result, together with (S35), can be plugged into (S31) to obtain the covariances of the other variables. As an example we report here the variance along the $x_2$ direction:

$$
\begin{aligned}
\left\langle (x_2 - \langle x_2 \rangle)^2 \right\rangle = {} & 2t\,\frac{D_{22}D_{33} - D_{23}^2}{D_{33}} + \frac{D_{23}^2}{D_{33}^2}\Bigg\{ \left[2D_{33} + v_3\left(x_3^{(0)} + v_3 t\right)\right]\sqrt{\frac{D_{33}t}{\pi v_3^2}}\, e^{-\frac{\left(x_3^{(0)} + v_3 t\right)^2}{4D_{33}t}} + \frac{D_{33}^2}{v_3^2}\,\mathrm{erfc}\left(\frac{x_3^{(0)} + v_3 t}{\sqrt{4D_{33}t}}\right) \\
& + \frac{1}{2}\left[2D_{33}t + \left(x_3^{(0)} + v_3 t\right)^2\right]\left(1 + \mathrm{erf}\left[\frac{x_3^{(0)} + v_3 t}{\sqrt{4D_{33}t}}\right]\right) - \left[D_{33} + v_3\left(x_3^{(0)} - v_3 t\right)\right]\frac{D_{33}}{v_3^2}\, e^{-\frac{v_3 x_3^{(0)}}{D_{33}}}\,\mathrm{erfc}\left[\frac{x_3^{(0)} - v_3 t}{\sqrt{4D_{33}t}}\right] \\
& - \left(x_3^{(0)} + v_3 t + \sqrt{\frac{D_{33}t}{\pi}}\, e^{-\frac{\left(x_3^{(0)} + v_3 t\right)^2}{4D_{33}t}} + \frac{D_{33}}{2v_3}\, e^{-\frac{v_3}{D_{33}}x_3^{(0)}}\,\mathrm{erfc}\left[\frac{x_3^{(0)} - v_3 t}{\sqrt{4D_{33}t}}\right] - \frac{1}{2}\left(x_3^{(0)} + v_3 t + \frac{D_{33}}{v_3}\right)\mathrm{erfc}\left[\frac{x_3^{(0)} + v_3 t}{\sqrt{4D_{33}t}}\right]\right)^2 \Bigg\}
\end{aligned}
\tag{S39}
$$

### B. Long time limit of the moments

The long-time limits can be obtained directly from the full time-dependent expressions or they can be derived by plugging the stationary distribution for $p(x_3)$ into the averages (S29) and (S31). By noticing that $\lim_{t\to\infty}\langle x_3 \rangle = -\frac{D_{33}}{v_3}$ and $\lim_{t\to\infty}(\langle x_3^2 \rangle - \langle x_3 \rangle^2) = \frac{D_{33}^2}{v_3^2}$ do not depend on time (as expected from the stationarity of the distribution) we

obtain

$$\lim_{t\to\infty}\frac{1}{t}\langle x_1\rangle = v_1 - \frac{D_{31}}{D_{33}}v_3\,, \tag{S40a}$$

$$\lim_{t\to\infty}\frac{1}{t}\langle x_2\rangle = v_2 - \frac{D_{32}}{D_{33}}v_3\,, \tag{S40b}$$

$$\lim_{t\to\infty}\frac{1}{t}\left(\langle x_1^2\rangle - \langle x_1\rangle^2\right) = 2\frac{D_{33}D_{11}-D_{31}^2}{D_{33}} = 2\tilde{D}_{11}\,, \tag{S40c}$$

$$\lim_{t\to\infty}\frac{1}{t}\left(\langle x_2^2\rangle - \langle x_2\rangle^2\right) = 2\frac{D_{33}D_{22}-D_{32}^2}{D_{33}} = 2\tilde{D}_{22}\,, \tag{S40d}$$

$$\lim_{t\to\infty}\frac{1}{t}\left(\langle x_1x_2\rangle - \langle x_1\rangle\langle x_2\rangle\right) = 2\frac{D_{33}D_{12}-D_{32}D_{31}}{D_{33}} = 2\tilde{D}_{12} \tag{S40e}$$

## III. ANISOTROPIC FRICTION

Anisotropic diffusion can not only be induced by an anisotropic thermal environment, but also by anisotropic friction. Such friction may be due to the particle's shape (non-spherical particles) or due to properties of the environment (e.g. intracellular media). However, anisotropic friction does not create non-equilibrium conditions such that it can not induce systematic motion along directions on which no force is applied. On a more formal level, the reason is that friction appears both in the diffusion and in the drift term via the fluctuation dissipation relation. The general situation describing anisotropic friction with isotropic temperatures is given by

$$\mathsf{D} = k_\mathrm{B}T\gamma^{-1} \tag{S41}$$

$$\boldsymbol{v} = \gamma^{-1}\boldsymbol{f} \tag{S42}$$

where $\boldsymbol{f} = (f_1, f_2, f_3)$. Inserting these relations into the result for the long-term drift (S40b) (eq. (8a) in the main text), we find

$$\langle\dot{x}_i\rangle = [(\gamma^{-1})_{33}(\gamma^{-1})_{ij}f_j - (\gamma^{-1})_{3i}(\gamma^{-1})_{3j}f_j]/(\gamma^{-1})_{33} \tag{S43}$$

for $i = 1$ or $i = 2$, i.e. for the components of motion parallel to the surface. This expression simplifies to become independent of $f_3$,

$$\langle\dot{x}_i\rangle = f_1[(\gamma^{-1})_{1i}(\gamma^{-1})_{33} - (\gamma^{-1})_{13}(\gamma^{-1})_{3i}]/(\gamma^{-1})_{33} + f_2[(\gamma^{-1})_{2i}(\gamma^{-1})_{33} - (\gamma^{-1})_{23}(\gamma^{-1})_{3i}]/(\gamma^{-1})_{33}\,. \tag{S44}$$

In other words, if we do not apply a force parallel to the surface, i.e. $f_1 = f_2 = 0$, then there will be no motion along the surface, $\langle\dot{x}_1\rangle = \langle\dot{x}_2\rangle = 0$, even though friction is anisotropic.

## IV. MODEL FOR THE EXPERIMENTAL PROPOSAL

We here discuss a few properties and an extension of the basic model used in the main text to describe the experimental set-up we propose in order to measure the transport effect predicted by our theory.

### A. Effective temperature

We demonstrate how the combination of isotropic thermal fluctuations and a fluctuating force with (almost) white noise characteristics can be modeled in terms of an anisotropic effective diffusion. In other words, we show how to pass from eq. (9) to eqs. (11a), (11b) in the main text. We start by multiplying eq. (9) of the main text by the inverse friction tensor to get

$$\dot{\boldsymbol{x}} = \gamma^{-1}\boldsymbol{f} + \sigma\gamma^{-1}\boldsymbol{e}_\sigma\zeta(t) + \sqrt{2k_\mathrm{B}T}\gamma^{-1/2}\boldsymbol{\xi}(t)\,. \tag{S45}$$

We recall that $\boldsymbol{\xi}(t) = (\xi_1(t), \xi_2(t), \xi_3(t))$ collects three unbiased, mutually independent Gaussian white noise sources (with $\langle \xi_i(t)\xi_j(t')\rangle = \delta_{ij}\delta(t-t')$), and that $\zeta(t)$ is an unbiased delta-correlated white noise, $\langle \zeta(t)\zeta(t')\rangle = \delta(t-t')$. Component-wise we have

$$\dot{x}_i = \left(\gamma^{-1}\right)_{ik} f_k + \underbrace{\sigma \left(\gamma^{-1}\right)_{ik} (\boldsymbol{e}_\sigma)_k \,\zeta(t) + \sqrt{2k_{\mathrm{B}}T}\left(\gamma^{-1/2}\right)_{ik} \xi_k(t)}_{s_i(t)}\,, \tag{S46}$$

where we see that there is a deterministic component $\left(\gamma^{-1}\boldsymbol{f}\right)_i$, and a stochastic one whose different terms we collect in $s_i(t)$. Actually, $s_i(t)$ is the sum of two independent Gaussian processes and thus is a Gaussian process as well. As such it is fully specified by its first and second moments. Since $\zeta(t)$ and $\xi_k(t)$ have zero average, also their sum (or any of their linear combinations) will have zero average, implying $\langle s_i\rangle = 0$. The covariance of the stochastic term is given by

$$\begin{aligned}\langle s_i(t)s_j(t')\rangle &= \sigma^2 \left(\gamma^{-1}\right)_{ik} (\boldsymbol{e}_\sigma)_k \left(\gamma^{-1}\right)_{jl} (\boldsymbol{e}_\sigma)_l \,\delta(t-t') + 2k_{\mathrm{B}}T \left(\gamma^{-1/2}\right)_{ik}\left(\gamma^{-1/2}\right)_{jl}\delta_{kl}\delta(t-t') \\ &= \left[\sigma^2(\gamma^{-1}\boldsymbol{e}_\sigma)_i(\gamma^{-1}\boldsymbol{e}_\sigma)_j + 2k_{\mathrm{B}}T\,(\gamma^{-1})_{ij}\right]\delta(t-t')\,.\end{aligned} \tag{S47}$$

To arrive at this final expression, we have exploited the symmetry of the friction tensor and the independence of $\zeta(t)$ and $\xi_k(t)$, i.e. $\langle \zeta(t)\xi_k(t')\rangle = 0$.

We can now replace the stochastic component $s_i(t)$ by a new, effective stochastic noise with identical statistical properties without changing the dynamics of the equation. This new noise process can be written as $\sqrt{2}\mathsf{D}^{1/2}\,\boldsymbol{\xi}_{\mathrm{eff}}(t)$, with $\boldsymbol{\xi}_{\mathrm{eff}}(t)$ again being unbiased Gaussian white noise sources $\langle \left(\xi_{\mathrm{eff}}\right)_i(t)\left(\xi_{\mathrm{eff}}\right)_j(t')\rangle = \delta_{ij}\delta(t-t')$, and with the effective diffusion tensor

$$D_{ij} = \frac{\sigma^2}{2}(\gamma^{-1}\boldsymbol{e}_\sigma)_i(\gamma^{-1}\boldsymbol{e}_\sigma)_j + k_{\mathrm{B}}T\,(\gamma^{-1})_{ij}\,, \tag{S48}$$

where $\mathsf{D}^{1/2}\mathsf{D}^{1/2} = \mathsf{D}$. With this definition of $\mathsf{D}$ it is obvious that the vector components $\left(\sqrt{2}\mathsf{D}^{1/2}\,\boldsymbol{\xi}_{\mathrm{eff}}(t)\right)_i$ have the same statistical properties as $s_i(t)$. It is then equivalent to express (S45) as

$$\dot{\boldsymbol{x}} = \gamma^{-1}\boldsymbol{f} + \sqrt{2}\mathsf{D}^{1/2}\,\boldsymbol{\xi}_{\mathrm{eff}}(t)\,, \tag{S49}$$

which, upon substitution of $\gamma^{-1}\boldsymbol{f} = \boldsymbol{v}$, gives eq. (10) in the main text.

### B. Properties of the long-term velocity

We here explore the dependence of the the long-term drift velocities on the "synthetic" temperature intensity and its direction. Their explicit expressions can be computed from the general expressions (S40), and, for the experimental set-up considered in the main text (see also previous Section), they read

$$\langle \dot{x}_1\rangle = f_1/\tilde{\gamma}, \tag{S50}$$

$$\langle \dot{x}_2\rangle = \frac{1}{\tilde{\gamma}}\left[f_2 - f_3\frac{\sin\theta\cos\theta}{\frac{T}{T_{\mathrm{kin}}-T}\frac{\tilde{\gamma}}{\gamma_0} + \sin^2\theta}\right]\,, \tag{S51}$$

where the angle $\theta$ defines the direction of the "synthetic" noise (see also Fig. 1 in the main text), and where we have introduced the standard definition $T_{\mathrm{kin}} = T + \frac{\sigma^2}{2k_{\mathrm{B}}\gamma_0}$ for the "hot" kinetic (or effective) temperature [1–3] with a "reference" friction coefficient $\gamma_0$, which we choose to be the Stokes friction coefficient of a spherical particle with radius $0.5\,\mu$m (for such a particle the properties of the synthetic noise have been analyzed in [1, 2]).

The friction coefficient of the actual particle which is moving along the surface is given by $\tilde{\gamma}$; for now we approximate it by Stokes friction in an unbounded fluid (corrections to this approximation due to hydrodynamic interactions between particle and surface are discussed in the next section). For fixed values of the force components $f_2$ and $f_3$, variations in the intensity and the direction of the "synthetic" temperature change the long-term drift velocity of the particle, which can even switch sign, see fig 2.

It is also possible to consider two particles of different sizes and compare the dependence of their net velocities on the temperature anisotropy. In fig. 3, we show the velocity (S51) of two spherical particles with different radii as a function of the the direction $\theta$ of the applied fluctuating force for fixed intensity $T_{\mathrm{kin}}$. This is useful for determining under what conditions the two particles will move into opposite directions.

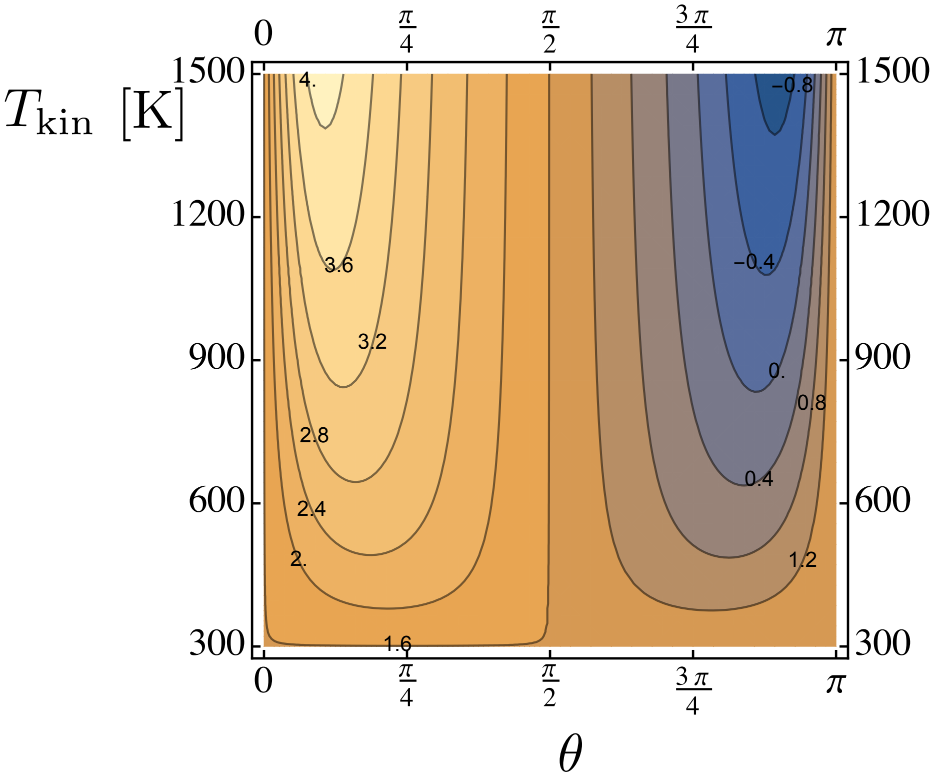


FIG. 2. Plot of $\langle \dot{x}_2 \rangle$, the long-term drift along $x_2$ (in $\mu$m s$^{-1}$ following eq. (S51)) for a particle of size $0.25\,\mu$m as a function of the "synthetic" kinetic temperature $T_{\rm kin} = T + \sigma^2/(2k_{\rm B}\gamma_0)$ (specified for a reference spherical particle with radius $0.5\,\mu$m and Stokes friction coefficient $\gamma_0$), and the direction $\theta$. The remaining parameters are those used for figure 1 in the main text: $T = 300\,$K, $\boldsymbol{f} = (0\,\text{fN}, 7.5\,\text{fN}, -9\,\text{fN})$. Warm (orange) colors denote positive values of $\langle \dot{x}_2 \rangle$, cold (blue) colors negative ones. The contours represent lines of constant $\langle \dot{x}_2 \rangle$ with the velocity values indicated.

We finally point out that the drift speed of the particle motion over the surface can be increased by simultaneously scaling up the forces $f_2$ and $f_3$. From the result (S51) we see that then the net particle velocity will be increased by the same factor. The particle dispersion, on the other hand, is not affected by $f_2$ and $f_3$ and thus stays the same; this follows from (S40c), (S40d), and (S40e). In that way, one would obtain perfect separation of the two particles from the main text after just 1 s by forces $f_2$ and $f_3$ which are scaled up by a factor 1000 to become of the order of pN.

However, for such large forces the particle is pressed extremely close towards the surface. In fact, the average gap between particle and surface $-D_{33}/v_3$ is of the order of 0.5 nm. This distance corresponds to the size of roughly two water molecules! It thus represents a situation in which not only neglecting the hydrodynamic interactions between the particle and the flat surface produces huge errors, but in which the whole modeling approach based on Langevin equations and continuous hydrodynamic descriptions breaks down. For forces in the range of fN, like used in the main text, the average gap size is about $0.5\,\mu$m. Including the hydrodynamic interactions between the particle and the plain surface, excellent agreement between experiments and a Langevin model has been reported for particle-wall gaps down to about 50 nm for particles with radius $2.5\,\mu$m, i.e. for gaps which are about 2% of the particle radius [10]. We therefore conclude that the Langevin description is trustworthy at least up to forces which are ten times larger than the ones used in the main text. However, for a quantitatively accurate prediction of the net particle velocities one would have to take into account the hydrodynamic interactions between the particle and the flat boundary.

### C. Hydrodynamic effects

It is well known that the main effect of hydrodynamic interactions between particles and walls is an increase of the viscous friction effects [8], where friction parallel and perpendicular to the surface are affected differently. In other words, the (inverse) friction coefficient becomes a tensor quantity with entries which are functions of the particle-

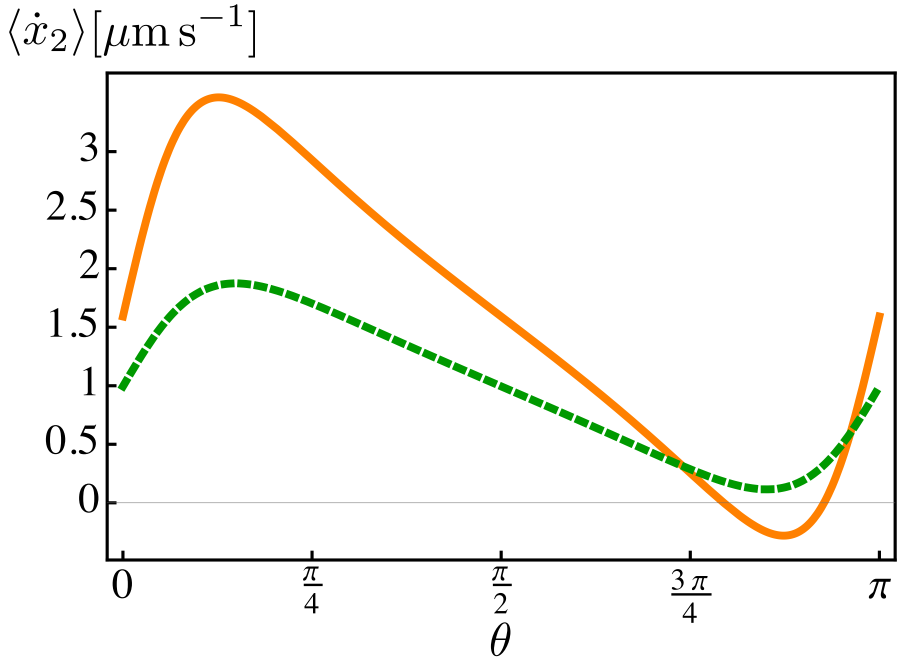


FIG. 3. Plot of $\langle \dot{x}_2 \rangle$, the long-term drift along $x_2$ (in $\mu$m s$^{-1}$ following eq. (S51)) for a particle of size $0.25\,\mu$m (solid orange curve) and for a particle of size $0.4\,\mu$m (dashed green curve) as a function of the direction $\theta$. The remaining parameters are those used for figure 1 in the main text: $T = 300\,$K, "synthetic" kinetic temperature $T_{\rm kin} = T + \sigma^2/(2k_{\rm B}\gamma_0) = 1000\,$K (specified for a reference spherical particle with radius $0.5\,\mu$m and Stokes friction coefficient $\gamma_0$), and $\boldsymbol{f} = (0\,{\rm fN}, 7.5\,{\rm fN}, -9\,{\rm fN})$.

surface gap $x_3$,

$$\gamma^{-1} = \begin{pmatrix} \mu_{\parallel}(x_3) & 0 & 0 \\ 0 & \mu_{\parallel}(x_3) & 0 \\ 0 & 0 & \mu_{\perp}(x_3) \end{pmatrix} . \tag{S52}$$

The mobilities $\mu_{\parallel}(x_3)$ and $\mu_{\perp}(x_3)$ parallel and perpendicular to the surface actually depend on the ratio $\delta = (x_3+a)/a$ between distance $x_3 + a$ of the particle center from the wall and particle radius $a$, irrespective of particle size. They can be approximated with high accuracy by

$$\mu_{\parallel} = \frac{1}{\tilde{\gamma}} \left( 1 - \frac{9}{16\delta} + \frac{1}{8\delta^3} - \frac{45}{256\delta^4} - \frac{1}{16\delta^5} \right) , \tag{S53a}$$

$$\mu_{\perp} = \frac{1}{\tilde{\gamma}} \frac{6\delta^2 - 10\delta + 4}{6\delta^2 - 3\delta - 1} , \tag{S53b}$$

with $\tilde{\gamma} = 6\pi\nu a$ being the Stokes friction coefficient of the spherical particle in a unbounded fluid (viscosity $\nu$). The first expression is an expansion of the exact $\mu_{\parallel}$ up to fifth order in $\delta$ (see formula (7-4.28) in [8]). The second expression is a fit to the exact result for $\mu_{\perp}$, which is known in terms of an infinite sum (see formula (7-4.38) in [8]). This fit formula can, for instance, be found in [10, 11] (see also [12]); its relative error is below 1% in the whole range $\delta \in [1, \infty)$.

As a consequence of the $x_3$ dependence of the inverse friction coefficient (S52), the noise terms in (S45) are multiplicative, such that it is necessary to specify the prescription for their regularization. For multiplicative thermal noise with space-dependent friction it is established theoretically [13–17] and experimentally [18, 19] that the correct regularization is anti-Ito (also called Hänggi-Klimontovich [21, 22]). As for the synthetic noise we have to recall that it actually has a tiny, but finite correlation time [2, 20] which is sent to zero in the idealized model (S45), such that it has to be interpreted in the Stratonovich convention [23, 24]. Compensating these noise regularizations by "spurious" drift terms, we can rewrite the Langevin equation in Ito-form and then transform it into an equivalent equation with an anisotropic diffusion tensor, exactly like we did when recasting (S45) to (S49). The resulting Langevin equation

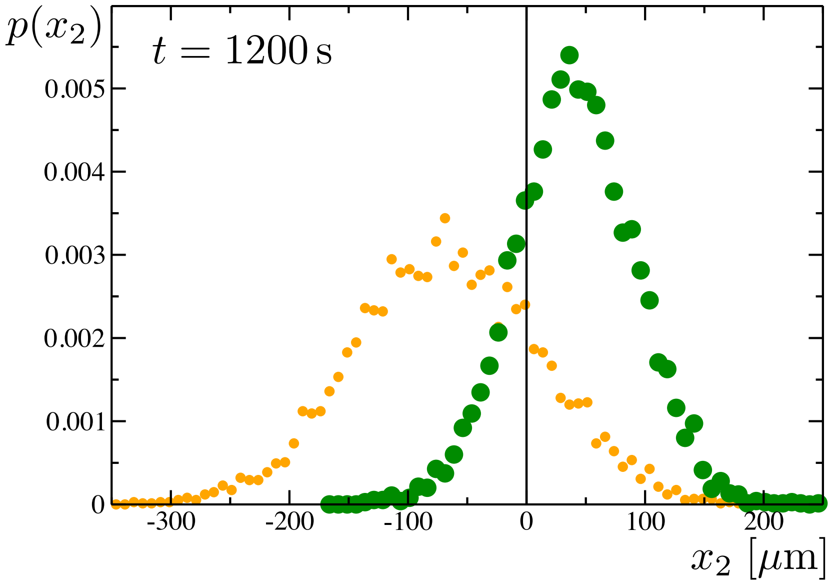


FIG. 4. Effect of hydrodynamic particle-surface interaction on the motion of the two different spherical particles from the main text along opposite directions on the surface. Small orange dots: Brownian sphere with radius $0.25\,\mu$m; large green dots: Brownian sphere with radius $0.4\,\mu$m. Shown are the probability densities $p(x_2) = \int_{-\infty}^{+\infty} \mathrm{d}x_1 \int_0^{+\infty} \mathrm{d}x_3\, p(x_1, x_2, x_3)$ for the two particles, obtained from numerically solving (S54) with (S52), (S53) and simulating 10000 realization of each particle species up to time $t = 1200\,\mathrm{s}$. Parameters are the same as in the main text, except for the force component $f_2$: $T = 300\,\mathrm{K}$ (room temperature), $T_{\mathrm{kin}} = T + \sigma^2/(2k_{\mathrm{B}}\gamma_0) = 1000\,\mathrm{K}$ ("synthetic" kinetic temperature, specified for a reference spherical particle with radius $0.5\,\mu$m and Stokes friction coefficient $\gamma_0$), $\theta = 0.9\pi$, $\boldsymbol{f} = (0\,\mathrm{fN}, 1.2\,\mathrm{fN}, -9\,\mathrm{fN})$.

reads

$$\dot{\boldsymbol{x}} = \gamma^{-1}\boldsymbol{f} + \frac{\sigma^2}{2a}\mu_\perp \sin\theta\cos\theta\,\mu_\parallel'\boldsymbol{e}_2 + \frac{1}{a}\left(k_{\mathrm{B}}T + \frac{\sigma^2}{2}\mu_\perp\sin^2\theta\right)\mu_\perp'\boldsymbol{e}_3 + \sqrt{2}\mathsf{D}^{1/2}\,\boldsymbol{\xi}_{\mathrm{eff}}(t)\,, \tag{S54}$$

where the prime denotes the derivative with respect to $\delta$ and the $\boldsymbol{e}_i$ are unit vectors along direction $x_i$. The diffusion tensor $\mathsf{D}$ is the same as before, see (S48).

Via $\mu_\parallel$ and $\mu_\perp$ the net drift forces now depend on position, such that an exact, time-dependent solution of the associated Fokker-Planck equation is not straightforward. Instead, we performed numerical simulations of the Langevin equation (S54) using essentially the same parameters as in the main text for the model without hydrodynamic interactions, see fig. 4. We find a qualitatively similar behavior as for that simpler model, but of course with changes in the exact quantitative behavior. In particular we had to adjust the exact value of the constant force component $f_2$ parallel to the surface to induce net movement of the two particle species into opposite directions. Although the simulation time is the same as in figure 1 of the main paper (1200 s), the two particles are less well separated, i.e. the sorting efficiency is smaller as compared to the case without hydrodynamic interactions. The main reason is that the increase of viscous friction with decreasing distance from the surface slows down the movement of the particles. A more quantitative analysis will be done in a future project.


[1] I. A. Martínez, É. Roldán, L. Dinis, and R. A. Rica, Soft Matter (2016).

[2] I. A. Martínez, É. Roldán, J. M. R. Parrondo, and D. Petrov, Phys. Rev. E **87**, 032159 (2013).

[3] L. Dinis, I. A. Martínez, É. Roldán, J. M. R. Parrondo, and R. A. Rica, J. Stat. Mech.: Theo. Exp. (2016), 054003.

[4] H. Behringer and R. Eichhorn, Phys. Rev. E **83**, 065701(R) (2011).

[5] H. Behringer and R. Eichhorn, J. Chem. Phys. **137**, 164108 (2012).

[6] M. V. Smoluchowski, Phys. Z. **17**, 557 (1916).

[7] S. Chandrasekhar, Rev. Mod. Phys. **15**, 1 (1943).
[8] J. Happel and H. Brenner, *Low Reynolds number hydrodynamics* (Martinus Nijhoff Publishers, The Hague, 1983).
[9] E. W. Ng, and M. Geller, A table of integrals of the error functions. Journal of Research of the National Bureau of Standards B, 73(1), 1-20. (1969).
[10] D. S. Sholl, M. K. Fenwick, E. Atman and D. C. Prieve, J. Chem. Phys. **113**, 9268 (2000).
[11] M. A. Bevan and D. C. Prieve, J. Chem. Phys. **113**, 1228 (2000).
[12] The slightly different functional form of (S53b) compared to the expressions in [10, 11] results from the fact that we write $\mu_\perp$ as a function of $\delta = (x_3 + a)/a$ rather than $x_3$. Note that our $x_3$ corresponds to the quantity $h$ in [10, 11].
[13] D. Ryter, Z. Phys. B **41**, 39 (1981).
[14] J. M. Sancho, M. San Miguel and D. Dürr, J. Stat. Phys. **28**, 291 (1982).
[15] A. M. Jayannavar and M. C. Mahato, Pramana J. Phys. **45**, 369 (1995).
[16] S. Hottovy, G. Volpe and J. Wehr, J. Stat. Phys. **146**, 762 (2012).
[17] M. Yang and M. Ripoll, Phys. Rev. E **87**, 062110 (2013).
[18] G. Volpe, L. Helden, T. Brettschneider, J. Wehr, and C. Bechinger, Phys. Rev. Lett. **104**, 170602 (2010).
[19] T. Brettschneider, G. Volpe, L. Helden, J. Wehr, and C. Bechinger, Phys. Rev. E **83**, 041113 (2011).
[20] P. Mestres, I. A. Martínez, A. Ortiz-Ambriz, R. A. Rica, and É. Roldán, Phys. Rev. E **90**, 032116 (2014).
[21] P. Hänggi and H. Thomas, Phys. Rep. **88**, 207 (1982).
[22] Yu. L. Klimontovich, Physics-Uspekhi **38**, 37 (1994).
[23] S. Bo and A. Celani, Phys. Rev. E **88**, 062150 (2013).
[24] C. W. Gardiner, *Handbook of Stochastic Methods for Physics, Chemistry and the Natural Sciences* (Springer, Berlin, 1985).
